# Supplementary material for: Confinement- and strain-induced enhancement of thermoelectric properties in LaNiO$_3$/LaAlO$_3(001)$ superlattices
Source: arXiv:1804.07070 ancillary file (2018-05-11)
Supplement: Supplementary file 1 [file Supplement.pdf]

# Confinement- and strain-induced enhancement of thermoelectric properties in $LaNiO_3/LaAlO_3(001)$ superlattices
# – Supplemental Material –

Benjamin Geisler and Rossitza Pentcheva
*Fakultät für Physik, Universität Duisburg-Essen and Center for Nanointegration (CENIDE), Campus Duisburg, Lotharstr. 1, 47048 Duisburg, Germany*

## I. STRUCTURAL INFORMATION

### A. $(LNO)_1/(LAO)_1(001)$ superlattices

Tables I and II summarize structural aspects of the 1/1 SLs. Increasing the substrate lattice constant $a$ and hence the epitaxial strain $\epsilon = a/a_{\mathrm{LNO}} - 1$ leads to a reduced cell height $c$. This is directly reflected by the La-La distances in the $[001]$ direction, which reduce with the lateral strain and are similar across a $NiO_2$ layer and across an $AlO_2$ layer (Table I). The $NiO_6$ and $AlO_6$ octahedral volumes show the general trend to increase with the epitaxial strain. For the $NiO_6$ octahedra, this trend is superimposed with the disproportionation effect, which enlarges (shrinks) those octahedra that enclose a larger (smaller) Ni magnetic moment. This interplay of electronic and structural disproportionation is also reflected by the O-$B$-O distances. In contrast, we find only minor volume differences between neighboring $AlO_6$ octahedra; these are caused by their direct connection to the $NiO_6$ octahedra.

The basal (i.e., in-plane) bond angles provided in Table II remain close to their respective bulk values for all degrees of epitaxial strain considered here. In contrast, the apical (out-of-plane) angles decrease considerably with increasing epitaxial strain, i.e., the structure gets tilted more strongly. This can also be observed by closely inspecting the structural models shown in Fig. 1 in the paper.

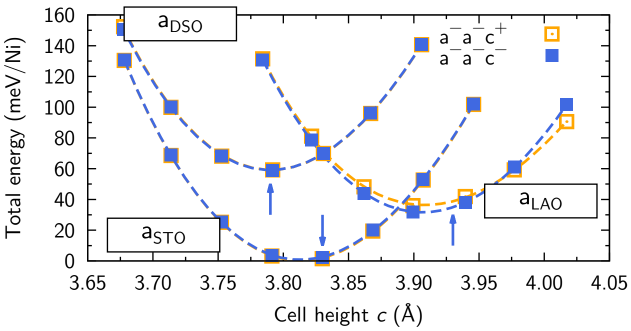


Figure 1. Total energy curves of $(LNO)_1/(LAO)_1(001)$ SLs as functions of $c$ for compressive ($a_{\mathrm{LAO}}$, right) and tensile ($a_{\mathrm{STO}}$ and $a_{\mathrm{DSO}}$, left) epitaxial strain and two different octahedral tilting patterns. The $c$ values used by us are marked by arrows. For $a_{\mathrm{LAO}}$ and $a_{\mathrm{STO}}$, the literature values we used for consistency are close to our optimized values (energy minima). The degeneracy of the two $a_{\mathrm{STO}}$ (and $a_{\mathrm{DSO}}$) curves is caused by the vanishing rotation of the $AlO_6$ octahedra around the $c$ axis. Moreover, the curves show that SL growth on STO is more relaxed than on DSO or LAO.

For $a_{\mathrm{LAO}}$, we found the ground-state octahedral rotation pattern to be $a^-a^-c^-$ (Fig. 1). The rotations of the $AlO_6$ octahedra around the $c$ axis are driven out for $a_{\mathrm{STO}}$ and $a_{\mathrm{DSO}}$, whereas those around the $a$ axes increase relative to the case of $a_{\mathrm{LAO}}$. Hence, the distinction between $a^-a^-c^-$ and $a^-a^-c^+$ octahedral rotation patterns is not useful for $a_{\mathrm{STO}}$ and $a_{\mathrm{DSO}}$. The $NiO_6$ octahedra exhibit significant tilts around all three axes for all considered degrees of epitaxial strain.

### B. $(LNO)_3/(LAO)_3(001)$ superlattices

For the 3/3 SLs, the La-La distances reflect more strongly the type of bridged $BO_2$ layer as for the 1/1 SLs, decreasing significantly from central $NiO_2$ to central $AlO_2$ (by $-3.3\,\%$ and $-2.6\,\%$ for $a_{\mathrm{LAO}}$ and $a_{\mathrm{STO}}$, respectively, the bulk difference just being $-1.3\,\%$; cf. Table III). The O-Ni-O distances show that the $NiO_6$ octahedra are elongated in the $[001]$ direction by about $4\,\%$ for $a_{\mathrm{LAO}}$, in particular at the interface. In contrast, for $a_{\mathrm{STO}}$, they are more regular and even slightly compressed at the interface. The $AlO_6$ octahedra are elongated (compressed) in the $[001]$ direction for $a_{\mathrm{LAO}}$ ($a_{\mathrm{STO}}$) and equally sized in all layers. Their volume is similar to that in the 1/1 SLs and larger for $a_{\mathrm{STO}}$ than for $a_{\mathrm{LAO}}$. The $NiO_6$ octahedral volumes are generally larger than the $AlO_6$ ones (as are the bulk values), and for the 3/3 SLs they are larger than for the 1/1 SLs (averaged).

The different degree of octahedral tilting between compressive and tensile strain is more clearly visible for the 3/3 SLs than for the 1/1 SLs, as one can infer also from the structural models shown in Figs. 1 and 5 in the paper. In general, the basal Ni-O-Ni bond angles are smaller (i.e., stronger tilts) for both $a_{\mathrm{LAO}}$ and $a_{\mathrm{STO}}$ as for the 1/1 SLs, and further away from the LNO bulk value (Table III). The Ni-related apical bond angles exhibit a slightly higher responsiveness to epitaxial strain (i.e., a larger difference comparing $a_{\mathrm{LAO}}$ and $a_{\mathrm{STO}}$ values) for the 3/3 SLs as for the 1/1 SLs (Table II).

Similar to the case of the 1/1 SLs, the $AlO_6$ octahedra exhibit almost no rotation around the $c$ axis for 3/3 SLs at $a_{\mathrm{STO}}$ and $a_{\mathrm{DSO}}$, whereas the rotations around the $a$ axes increase relative to the case of $a_{\mathrm{LAO}}$. The $NiO_6$ octahedra exhibit significant tilts around all three axes for all considered degrees of epitaxial strain. We found that the ground-state octahedral rotation pattern is $a^-a^-c^-$ for both $a_{\mathrm{LAO}}$ and $a_{\mathrm{STO}}$. For $a_{\mathrm{LAO}}$, an initial $a^-a^-c^+$ pattern relaxed directly to $a^-a^-c^-$. For $a_{\mathrm{STO}}$, an initial $a^-a^-c^+$ pattern relaxed to a quasi $a^-a^-c^0$ pattern, which is by 32 meV/f.u. less stable than $a^-a^-c^-$.

Table I. Site-resolved O-$B$-O distances, La-La distances in the [001] direction, $NiO_6$ and $AlO_6$ octehadral volumes, and Ni spin magnetic moments of $(LNO)_1/(LAO)_1(001)$ SLs for different degrees of epitaxial strain $\epsilon = a/a_{LNO} - 1$. For the bulk values, experimental cell parameters and optimized internal coordinates have been used.

| | $\epsilon$ (%) | O-$B$-O distance (Å) | | La-La distance (Å) | | $B$O$_6$ octahedral volume (Å$^3$) | | Local mag. mom. ($\mu_B$) |
|---|---|---|---|---|---|---|---|---|
| | | Ni1 / Ni2, basal | Ni1 / Ni2, apical | @ $NiO_2$ | @ $AlO_2$ | Ni1 / Ni2 | Al1 / Al2 | Ni1 / Ni2 |
| $a_{LAO}$ | −1.2 | 3.82 / 3.85 | 3.98 / 4.05 | 3.94 | 3.92 | 9.65 / 10.02 | 9.47 / 9.44 | 0.89 / 1.17 |
| $a_{STO}$ | +1.7 | 3.86 / 4.04 | 3.86 / 3.98 | 3.83 | 3.84 | 9.60 / 10.84 | 9.82 / 9.83 | 0.60 / 1.41 |
| $a_{DSO}$ | +2.7 | 3.89 / 4.13 | 3.88 / 3.99 | 3.80 | 3.80 | 9.79 / 11.32 | 9.92 / 9.98 | 0.54 / 1.46 |
| $LaNiO_3$ | | 3.89 | | 3.84 | – | 9.80 | – | 1.04 |
| $LaAlO_3$ | | 3.81 | | – | 3.79 | – | 9.23 | – |

Table II. $B$-O-$B$ bond angles of $(LNO)_1/(LAO)_1(001)$ SLs for different degrees of epitaxial strain. The bulk values have been obtained as described in Table I.

| | basal (°) | | apical (°) | |
|---|---|---|---|---|
| | Ni1-O-Ni2 | Al1-O-Al2 | Ni1-O-Al1 | Ni2-O-Al2 |
| $a_{LAO}$ | 162 | 167 | 166 | 167 |
| $a_{STO}$ | 162 | 168 | 162 | 164 |
| $a_{DSO}$ | 159 | 166 | 156 | 159 |
| $LaNiO_3$ | 161 | – | – | – |
| $LaAlO_3$ | – | 168 | – | – |

## II. REVIEW OF DIFFERENT THERMOELECTRIC OXIDE SYSTEMS

The following experimental and theoretical results obtained around room temperature for a selection of different oxide systems have been summarized in Table I of the paper.

Okuda *et al.* investigated the effect of La doping in STO.[1] They reported $S = -380$ $\mu$V/K for (almost) pure STO and a power factor of 2.5 $\mu$W/K$^2$cm. For an increased La percentage, the Seebeck coefficient lowers to $-260$ $\mu$V/K, but the power factor reaches its maximum of 35 $\mu$W/K$^2$cm.

Hybrid functional calculations by Bilc *et al.*[2] for bulk STO using $\tau = 4.3$ fs lead to $-77$ $\mu$V/K, 10 $\mu$W/K$^2$cm and $-400$ $\mu$V/K, 3 $\mu$W/K$^2$cm for $n$-type carrier concentrations of $n = 10^{19}$ and $10^{21}$/cm$^3$, respectively.

Jalan and Stemmer studied La-doped STO thin films on STO(001) and LSAT(001) substrates.[3] With increasing carrier concentration ($n = 2 \cdot 10^{19}$, $2 \cdot 10^{20}$, and $7 \cdot 10^{20}$/cm$^3$) they report decreasing Seebeck coefficients of $-600$, $-300$, and $-200$ $\mu$V/K, but strongly increasing power factors of 7, 24, and 39 $\mu$W/K$^2$cm, respectively, due to an exponentially increasing electrical conductivity. Lower doping leads to a Seebeck coefficient of $-980$ $\mu$V/K. For La-$\delta$-doped STO SLs they measured Seebeck coefficients of about $-500$ $\mu$V/K.

Lemal *et al.* performed hybrid functional calculations for pristine CCO and used $\tau = 0.8$ fs.[4] For a carrier concentration of $n = 10^{18}$/cm$^3$ they found in-plane Seebeck coefficients of about $-500$ $\mu$V/K for $n$-type doping and about $+700$ $\mu$V/K for $p$-type doping at room temperature. The maximal power factor of around 0.7 $\mu$W/K$^2$cm was reached close to $n = 10^{21}$/cm$^3$.

Amin *et al.*[5] studied CCO by using DFT+$U$ calculations and found a strong dependence of Seebeck coefficient and power factor on epitaxial strain, ranging in-plane from +25 to +100 $\mu$V/K and from 0.3 to 0.6 $\mu$W/K$^2$cm at room temperature. (The values in Table I in the paper refer to $a_{STO}$.) Their cross-plane results are much lower. They used a relaxation time of $\tau = 0.3$ fs.

Yordanov *et al.*[6] explored the in-plane thermoelectric response of CCO on different perovskite substrates and found a strong increase of Seebeck coefficient and power factor on STO(001) and LAO(001) for temperatures above 725 K. Around room temperature, they report a Seebeck coefficient of about +150 $\mu$V/K and a power factor of 3 $\mu$W/K$^2$cm for 27 nm thick CCO films on STO(001).

Table III. Layer-resolved O-$B$-O distances, La-La distances in the [001] direction, $NiO_6$ and $AlO_6$ octehadral volumes, $B$-O-$B$ bond angles, and Ni spin magnetic moments of $(LNO)_3/(LAO)_3(001)$ SLs for different degrees of epitaxial strain. The bulk values have been obtained as described in Table I.

| | | Ni @ C | Ni @ IF | Al @ IF | Al @ C |
|---|---|---|---|---|---|
| O-$B$-O distance (Å) | | | | | |
| $a_{LAO}$ | basal | 3.87 | 3.87 | 3.81 | 3.81 |
| $a_{STO}$ | basal | 3.98 | 3.97 | 3.93 | 3.93 |
| $a_{LAO}$ | apical | 4.00 | 4.04 | 3.88 | 3.88 |
| $a_{STO}$ | apical | 4.01 | 3.93 | 3.81 | 3.81 |
| $LaNiO_3$ | | 3.89 | | – | |
| $LaAlO_3$ | | – | | 3.81 | |
| La-La distance across $B$O$_2$ layer (Å) | | | | | |
| $a_{LAO}$ | | 3.99 | 3.97 | 3.89 | 3.86 |
| $a_{STO}$ | | 3.88 | 3.86 | 3.81 | 3.78 |
| $LaNiO_3$ | | 3.84 | | – | |
| $LaAlO_3$ | | – | | 3.79 | |
| $B$O$_6$ octahedral volume (Å$^3$) | | | | | |
| $a_{LAO}$ | | 10.00 | 10.06 | 9.40 | 9.39 |
| $a_{STO}$ | | 10.54 | 10.33 | 9.80 | 9.79 |
| $LaNiO_3$ | | 9.80 | | – | |
| $LaAlO_3$ | | – | | 9.23 | |
| $B$-O-$B$ bond angle (°) | | | | | |
| $a_{LAO}$ | basal | 156 | 157 | 167 | 167 |
| $a_{STO}$ | basal | 158 | 159 | 167 | 168 |
| $a_{LAO}$ | apical | 168 | 168 | 168 | |
| $a_{STO}$ | apical | 161 | 160 | 163 | |
| $LaNiO_3$ | | 161 | | – | |
| $LaAlO_3$ | | – | | 168 | |
| Local magnetic moment ($\mu_B$) | | | | | |
| $a_{LAO}$ | | 1.03 | 1.06 | – | – |
| $a_{STO}$ | | 1.18 | 1.05 | – | – |
| $LaNiO_3$ | | 1.04 | | – | – |

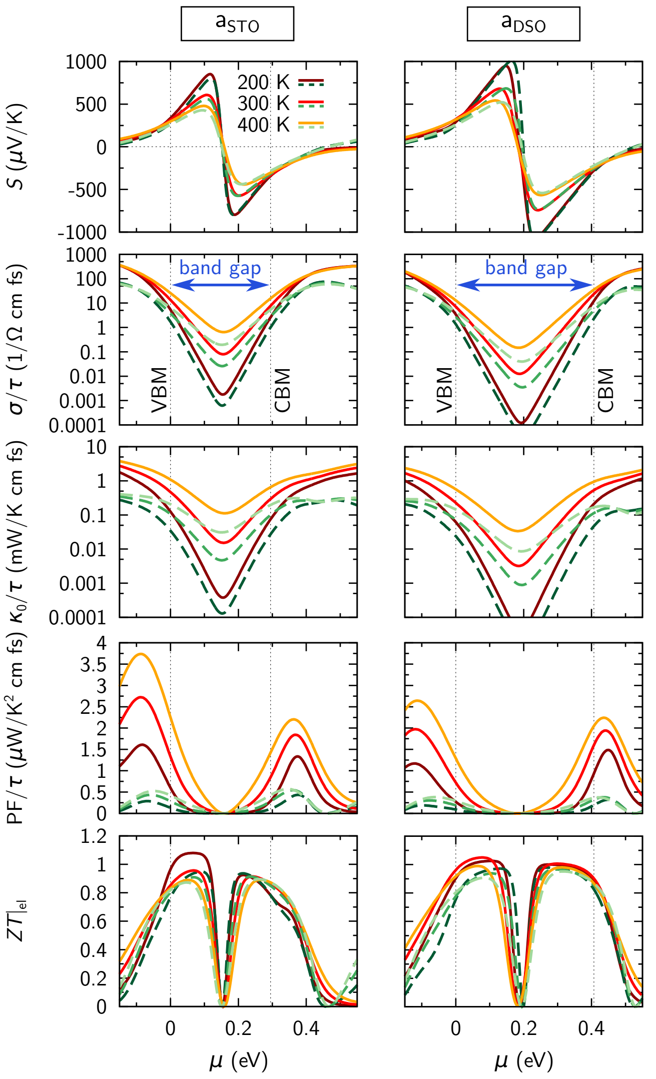


Figure 2. Thermoelectric properties of $(LNO)_1/(LAO)_1(001)$ SLs for different degrees of tensile strain ($a_{STO} < a_{DSO}$) at three different temperatures. Red-orange solid (green dashed) lines depict in-plane (cross-plane) transport. Note the larger band gap of 0.41 eV for $a_{DSO}$ (0.29 eV for $a_{STO}$).

## III. IMPACT OF TENSILE STRAIN BEYOND STO

Figure 2 compares the thermoelectric properties of $(LNO)_1/(LAO)_1(001)$ SLs for $a_{STO}$ and $a_{DSO}$ substrate lattice parameters, i.e., imposing two different degrees of tensile strain. We find that the maximally attainable Seebeck coefficient $S$ increases with strain, whereas the conductivities $\sigma$ and $\kappa_0$ as well as the power factor PF decrease. The reduced $\kappa_0$ stabilizes the electronic figure of merit $ZT|_{el}$. Nevertheless, we conclude that the thermoelectric response is better on STO, particularly in-plane.

## IV. OBTAINING ELECTRONIC TRANSPORT AND THERMOELECTRIC PROPERTIES FROM THE DFT ELECTRONIC STRUCTURE

We obtain the thermoelectric properties in linear response by using the approach of Sivan and Imry.[7] The central quantity is the energy- and spin-resolved transmission (transport distribution) $\mathcal{T}_\sigma(E)$ which we calculate by using the the BoltzTraP code.[8]

From the *ab initio* electronic structure $\varepsilon_{i,\vec{k},\sigma}$ we start by calculating the group velocities in different directions $\vec{e}$,

$$v_{i,\vec{k},\sigma} = \frac{1}{\hbar}\,\vec{e}\cdot\vec{\nabla}_k\,\varepsilon_{i,\vec{k},\sigma},$$

which we use to define the energy- and spin-resolved transmission in the corresponding direction,

$$\mathcal{T}_\sigma(E) = \frac{e^2}{N}\sum_{i,\vec{k}}\delta(E-\varepsilon_{i,\vec{k},\sigma})\left(v_{i,\vec{k},\sigma}\right)^2,$$

where $N$ is the total number of calculated $\vec{k}$ points. Within the common approximation of constant relaxation time $\tau$, the electrical conductivity can be expressed as

$$\sigma_\sigma(T,\mu) = -\frac{\tau}{\Omega}\int \mathrm{d}E\,\frac{\partial f}{\partial E}\,\mathcal{T}_\sigma(E),$$

where $\Omega = a^2 c$ is the volume of the considered supercell and $f = f_{\mu,T}(E)$ denotes the Fermi distribution function. The total conductivity is simply $\sigma = \sigma_\uparrow + \sigma_\downarrow$. Consequently, the SL conductivities presented in this work are normalized to the whole SL including the LAO regions, instead of to the LNO regions only as, for instance, in Ref. 9. The spin-projected Seebeck coefficients take on the form

$$S_\sigma(T,\mu) = -\frac{1}{eT}\,\frac{\int \mathrm{d}E\,\frac{\partial f}{\partial E}\,(E-\mu)\,\mathcal{T}_\sigma(E)}{\int \mathrm{d}E\,\frac{\partial f}{\partial E}\,\mathcal{T}_\sigma(E)}.$$

With these quantities the effective (charge) Seebeck coefficient can be expressed as

$$S = \frac{\sigma_\uparrow S_\uparrow + \sigma_\downarrow S_\downarrow}{\sigma_\uparrow + \sigma_\downarrow},$$

treating the two spin channels as parallel connected resistors. This provides the power factor $\mathrm{PF} = \sigma S^2$.

Finally, the transmission allows also to calculate the electronic contribution to the thermal conductivity,

$$\kappa_0(T,\mu) = -\frac{\tau}{e^2 T\Omega}\int \mathrm{d}E\,\frac{\partial f}{\partial E}\,(E-\mu)^2\,\{\mathcal{T}_\uparrow(E)+\mathcal{T}_\downarrow(E)\},$$

which enters the electronic figure of merit $ZT|_{el} = \sigma S^2 T/\kappa_0$.

[1] T. Okuda, K. Nakanishi, S. Miyasaka, and Y. Tokura, Phys. Rev. B **63**, 113104 (2001).

[2] D. I. Bilc, C. G. Floare, L. P. Zârbo, S. Garabagiu, S. Lemal, and P. Ghosez, J. Phys. Chem. C **120**, 25678 (2016).

[3] B. Jalan and S. Stemmer, Appl. Phys. Lett. **97**, 042106 (2010).

[4] S. Lemal, J. Varignon, D. I. Bilc, and P. Ghosez, Phys. Rev. B **95**, 075205 (2017).

[5] B. Amin, U. Eckern, and U. Schwingenschlögl, Appl. Phys. Lett. **110**, 233505 (2017).

[6] P. Yordanov, P. Wochner, S. Ibrahimkutty, C. Dietl, F. Wrobel, R. Felici, G. Gregori, J. Maier, B. Keimer, and H.-U. Habermeier, Appl. Phys. Lett. **110**, 253101 (2017).

[7] U. Sivan and Y. Imry, Phys. Rev. B **33**, 551 (1986).

[8] G. K. H. Madsen and D. J. Singh, Comput. Phys. Commun. **175**, 67 (2006).

[9] F. Wrobel, A. F. Mark, G. Christiani, W. Sigle, H.-U. Habermeier, P. A. van Aken, G. Logvenov, B. Keimer, and E. Benckiser, Appl. Phys. Lett. **110**, 041606 (2017).
